# Supplementary material for: Leveraging Large Language Models to Obscure Code Stylometry: A Comparative Study of GPT-3.5 and GPT-4
Source: arXiv:2606.22306 source file (2026-06-21)
Supplement: Supplementary file 1 [file I_appendix.tex]

%======================================================================
% APPENDIX - FINAL VERSION
%======================================================================

% Place this command before your appendix sections.
\appendix

\section{Methods2Test Dataset JSON Structure}
\label{app:json_structure}

A.1 Methods2Test Dataset JSON Structure.

% The figure environment has been removed to prevent floating.
% The 'center' environment is used for alignment.
\begin{center}
    % \includesvg requires "\usepackage{svg}" in your preamble.
    % The width is set to \columnwidth to fit in a single column.
    % \includesvg[width=0.9\columnwidth]{images/JSON.svg}
    \includegraphics[width=0.9\columnwidth]{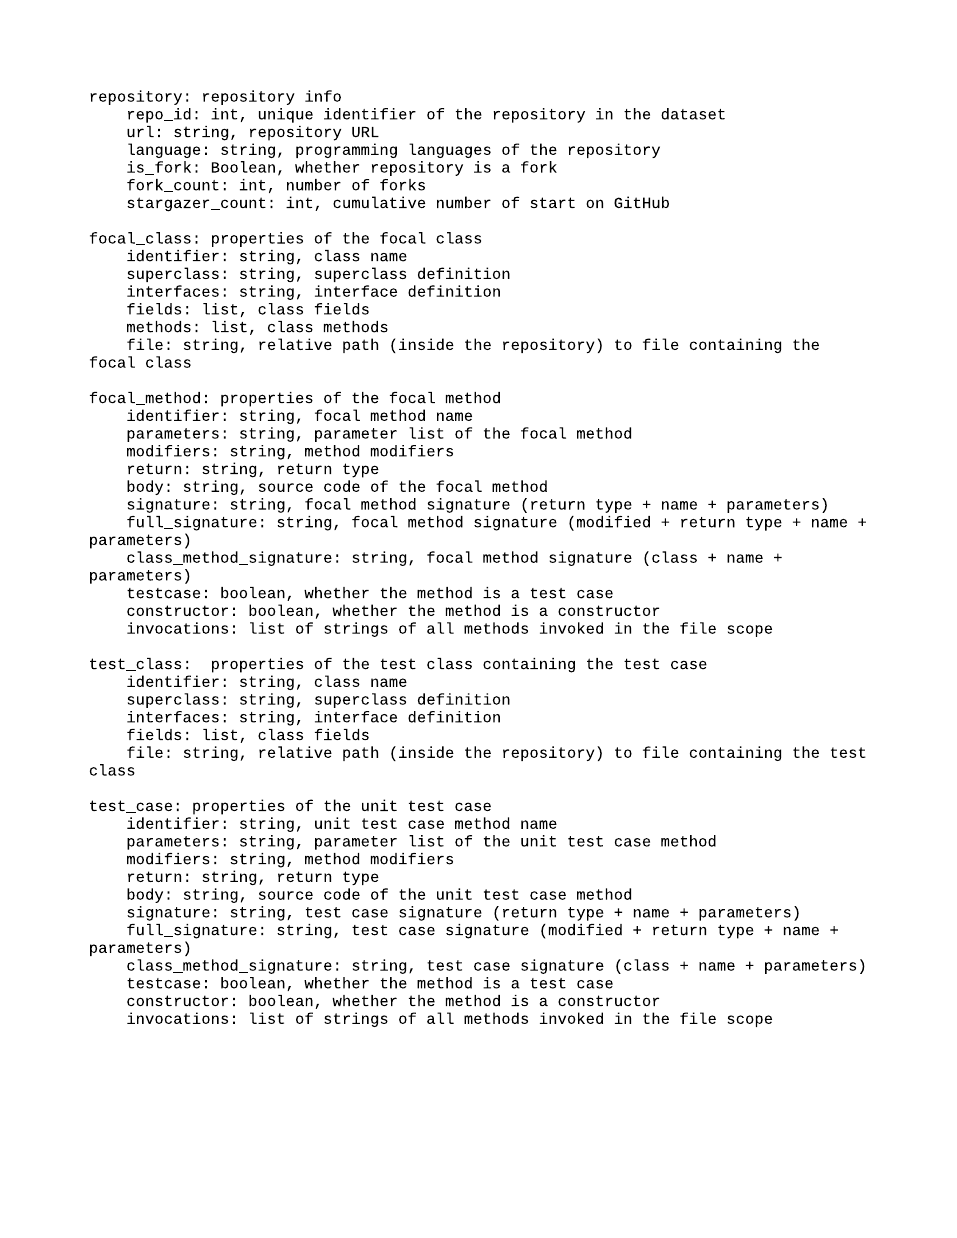}
    
    % The \captionof command adds a caption to a non-floating element.
    \captionof{figure}{Methods2Test Dataset JSON Structure.}
    \label{fig:JSON_structure}
\end{center}
